# Supplementary material for: Structure-Preserving Margin Distribution Learning for High-Order Tensor Data with Low-Rank Decomposition
Source: arXiv:2509.14577 source file (2025-09-18)
Supplement: Supplementary file 1 [file Appendix_SPMD-LRT.pdf]

## I. Appendix

### A. the SPMD-LRT Based on Rank-one Decomposition

For completeness, we outline the derivation when  $\mathcal{W}$  is constrained to a rank-1 tensor. Let

$$\mathcal{W} = \mathbf{w}^{(1)} \circ \mathbf{w}^{(2)} \circ \dots \circ \mathbf{w}^{(M)}, \quad (\text{A.1})$$

where each  $\mathbf{w}^{(m)}$  is an  $I_m$ -dimensional vector (the mode- $m$  factor). Then  $\langle \mathcal{W}, \mathcal{Z}_i \rangle = \prod_{m=1}^M (\mathbf{w}^{(m)T} \mathbf{z}_i^{(m)})$ , essentially the multi-linear form of the input with the factor vectors. The Frobenius norm  $\|\mathcal{W}\|_F^2$  simplifies to the product of the norms of each  $\mathbf{w}^{(m)}$ :

$$\begin{aligned} \|\mathcal{W}\|_F^2 &= \sum_{i_1=1}^{I_1} \sum_{i_2=1}^{I_2} \dots \sum_{i_M=1}^{I_M} \mathbf{w}_{i_1 i_2 \dots i_M}^2 \\ &= \sum_{i_1=1}^{I_1} \sum_{i_2=1}^{I_2} \dots \sum_{i_M=1}^{I_M} \left( \mathbf{w}_{i_1}^{(1)} \mathbf{w}_{i_2}^{(2)} \dots \mathbf{w}_{i_M}^{(M)} \right)^2 \\ &= \sum_{i_1=1}^{I_1} \dots \sum_{i_M=1}^{I_M} \prod_{m=1}^M \left[ \mathbf{w}^{(m)} \right]_{i_m}^2 \\ &= \prod_{i=1}^M \left\| \mathbf{w}^{(i)} \right\|_F^2 \\ &= \left\| \mathbf{w}^{(m)} \right\|_F^2 \prod_{\substack{i \neq m \\ 1 \leq i \leq M}} \left\| \mathbf{w}^{(i)} \right\|_F^2 \\ &= \eta \left\| \mathbf{w}^{(m)} \right\|_F^2 \end{aligned} \quad (\text{A.2})$$

The margin mean and variance for rank-1 SPMD-LRT become (analogous to Eq. (5) and (6) in main text, but now all modes are captured in the single outer-product form):

$$\begin{aligned} \gamma_m &= \frac{1}{N} \sum_{i=1}^N t_i \langle \mathcal{W}, \mathcal{Z}_i \rangle \\ &= \frac{1}{N} \sum_{i=1}^N t_i \left( \mathbf{w}^{(m)} \right)^T \mathbf{z}_i^m \\ &= \frac{1}{N} (\mathbf{Z}^m \mathbf{t})^T \mathbf{w}^{(m)} \end{aligned} \quad (\text{A.3})$$

$$\begin{aligned} \gamma_v &= \frac{1}{N} \sum_{i=1}^N (t_i \langle \mathcal{W}, \mathcal{Z}_i \rangle - \gamma_m)^2 \\ &= \frac{1}{N} \sum_{i=1}^N (t_i \langle \mathcal{W}, \mathcal{Z}_i \rangle)^2 - \left( \frac{1}{N} \sum_{i=1}^N t_i \langle \mathcal{W}, \mathcal{Z}_i \rangle \right)^2 \\ &= \frac{1}{N} \sum_{i=1}^N \left( t_i \left( \mathbf{w}^{(m)} \right)^T \mathbf{z}_i^m \right)^2 - \left( \frac{1}{N} (\mathbf{Z}^m \mathbf{t})^T \mathbf{w}^{(m)} \right)^2 \\ &= \left( \mathbf{w}^{(m)} \right)^T \mathbf{Z}^m \frac{N\mathbf{I} - \mathbf{t}\mathbf{t}^T}{N^2} (\mathbf{Z}^m)^T \mathbf{w}^{(m)} \end{aligned} \quad (\text{A.4})$$

Where  $\mathbf{Z}^m = [\mathbf{z}_1^m, \dots, \mathbf{z}_N^m]$  and  $\mathbf{t} = [t_1, \dots, t_N]$ . Substituting Eq. (A.2), Eq. (A.3) and Eq. (A.4) into Eq. (7), the problem becomes:

$$\begin{aligned} \min_{\mathbf{w}^{(m)}, \tau} \quad & \frac{\eta}{2} \left\| \mathbf{w}^{(m)} \right\|_F^2 + \left( \mathbf{w}^{(m)} \right)^T \mathbf{Z}^m \frac{\mu_1 (N\mathbf{I} - \mathbf{t}\mathbf{t}^T)}{N^2} \\ & (\mathbf{Z}^m)^T \mathbf{w}^{(m)} - \frac{\mu_2}{N} (\mathbf{Z}^m \mathbf{t})^T \mathbf{w}^{(m)} + \frac{\lambda}{N} \mathbf{e}^T \boldsymbol{\tau} \\ \text{s.t.} \quad & \mathbf{T} (\mathbf{Z}^m)^T \mathbf{w}^{(m)} \geq \mathbf{e} - \boldsymbol{\tau}, \boldsymbol{\tau} \geq 0 \end{aligned} \quad (\text{A.5})$$

where  $\mathbf{e}$  is all-one vector. Introducing the Lagrangian multipliers  $\alpha \geq 0$  and  $\beta \geq 0$ , the Lagrangian result of Eq. (A.5) is as follows:

$$L = \frac{1}{2} \left( \mathbf{w}^{(m)} \right)^T \mathbf{S} \mathbf{w}^{(m)} - \left( \mathbf{w}^{(m)} \right)^T \mathbf{Z}^m \mathbf{T} \left( \frac{\mu_2}{N} \mathbf{e} + \alpha \right) + \alpha^T \mathbf{e} + \tau^T \left( \frac{\lambda}{N} \mathbf{e} - \alpha - \beta \right) \quad (\text{A.6})$$

Where  $\mathbf{S} = \eta \left( \mathbf{I} + \mathbf{Z}^m \frac{2\mu_1(N\mathbf{I} - \mathbf{t}\mathbf{t}^T)}{\eta N^2} (\mathbf{Z}^m)^T \right)$ . By setting the partial derivative of  $\{\mathbf{w}^{(m)}, \tau\}$  to zero, we have:

$$\mathbf{w}^{(m)} = \mathbf{S}^{-1} \mathbf{Z}^m \mathbf{T} \left( \frac{\mu_2}{N} \mathbf{e} + \alpha \right), 0 \leq \alpha \leq \frac{\lambda}{N} \mathbf{e} \quad (\text{A.7})$$

By substituting Eq. (A.7) into Eq. (A.6), the dual of Eq. (A.5) can be cast as:

$$\begin{aligned} \min_{\alpha} \quad & \frac{1}{2} \left( \frac{\mu_2}{N} \mathbf{e} + \alpha \right)^T \mathbf{T} (\mathbf{Z}^m)^T \mathbf{S}^{-1} \mathbf{Z}^m \mathbf{T} \left( \frac{\mu_2}{N} \mathbf{e} + \alpha \right) - \mathbf{e}^T \alpha \\ \text{s.t.} \quad & 0 \leq \alpha \leq \frac{\lambda}{N} \mathbf{e} \end{aligned} \quad (\text{A.8})$$

According to the Sherman-Morrison-Woodbury formula, we have

$$\mathbf{S}^{-1} \mathbf{Z}^m = \frac{1}{\eta} \mathbf{Z}^m (\mathbf{I} + \mathbf{Q}\mathbf{G})^{-1} \quad (\text{A.9})$$

where  $\mathbf{Q} = \frac{2\mu_1(N\mathbf{I} - \mathbf{t}\mathbf{t}^T)}{\eta N^2}$  and  $\mathbf{G} = (\mathbf{Z}^m)^T \mathbf{Z}^m$ . Then  $(\mathbf{Z}^m)^T \mathbf{S}^{-1} \mathbf{Z}^m = \frac{1}{\eta} \mathbf{G} (\mathbf{I} + \mathbf{Q}\mathbf{G})^{-1}$ . By denoting  $\mathbf{H} = \frac{1}{\eta} \mathbf{T}\mathbf{G} (\mathbf{I} + \mathbf{Q}\mathbf{G})^{-1} \mathbf{T}$ , the objective function of Eq. (A.8) can be written as

$$f(\alpha) = \frac{1}{2} \alpha^T \mathbf{H} \alpha + \left( \frac{\mu_2}{N} \mathbf{H} \mathbf{e} - \mathbf{e} \right)^T \alpha + \text{const} \quad (\text{A.10})$$

After eliminating the constant term, which does not influence the optimization process, the final form of the SPMD-LRT is presented as follows:

$$\begin{aligned} \min_{\alpha} \quad & \frac{\alpha^T \mathbf{H} \alpha}{2} + \left( \frac{\mu_2}{N} \mathbf{H} \mathbf{e} - \mathbf{e} \right)^T \alpha \\ \text{s.t.} \quad & 0 \leq \alpha \leq \frac{\lambda}{N} \mathbf{e} \end{aligned} \quad (\text{A.11})$$

The coefficient  $\mathbf{w}^{(m)}$  can be derived from the result  $\alpha^*$  of the optimization problem Eq. (A.11) as follows:

$$\mathbf{w}^{(m)} = \mathbf{Z}^m \frac{1}{\eta} (\mathbf{I} + \mathbf{Q}\mathbf{G})^{-1} \mathbf{T} \left( \frac{\mu_2}{N} \mathbf{e} + \alpha^* \right) = \mathbf{Z}^m \mathbf{u} \quad (\text{A.12})$$

Where  $\mathbf{u} = \frac{1}{\eta} (\mathbf{I} + \mathbf{Q}\mathbf{G})^{-1} \mathbf{T} \left( \frac{\mu_2}{N} \mathbf{e} + \alpha^* \right)$ . It should be mentioned here that the whole procedure is repeated iteratively for every mode. The pseudo-code for the SPMD-LRT based on the Rank-1 decomposition (SPMD-LRT) is provided in Algorithm 2.

---

Algorithm 1 SPMD-LRT Algorithm

---

!htbp

Input: Training dataset  $\left\{ \mathcal{Z}_i \in \mathbb{R}^{I_1 \times I_2 \times \dots \times I_M}, \mathbf{t}_i \in \{-1, 1\}_{i=1}^N \right\}$ , Parameters:  $\mu_1, \mu_2, \lambda$ 

Output:  $\mathcal{W}$ 

Steps:

- 1: Set  $\mathbf{w}^{(m)}$  equal to random unit vector in  $\mathbb{R}^{I_m}$ .
- 2: Do Steps 3-5 until convergence.
- 3: For  $m = 1$  to  $M$
- 4: Update  $\mathbf{w}^{(m)}$  by the following question

$$\min_{\boldsymbol{\alpha}} \frac{\boldsymbol{\alpha}^T \mathbf{H} \boldsymbol{\alpha}}{2} + \left( \frac{\mu_2}{N} \mathbf{H} \mathbf{e} - \mathbf{e} \right)^T \boldsymbol{\alpha}$$

$$s.t. \ 0 \leq \boldsymbol{\alpha} \leq \frac{\lambda}{N} \mathbf{e}$$

Where  $\mathbf{w}^{(m)} = \mathbf{Z}^{m \frac{1}{\eta}} (\mathbf{I} + \mathbf{Q} \mathbf{G})^{-1} \mathbf{T} \left( \frac{\mu_2}{N} \mathbf{e} + \boldsymbol{\alpha}^* \right)$ 

5: End For

6: Convergence checking:

$$if \ \left\| \mathcal{W}^{(t)} - \mathcal{W}^{(t-1)} \right\| / \left\| \mathcal{W}^{(t-1)} \right\| \leq \varepsilon$$

Where  $\mathcal{W} = \mathbf{w}^{(1)} \circ \mathbf{w}^{(2)} \circ \dots \circ \mathbf{w}^{(M)} = \circ_{m=1}^M \mathbf{w}^{(m)}$ , the calculate  $\mathbf{w}^{(m)}, m = 1, 2, \dots, M$  have converged. Here  $\mathcal{W}^{(t)}$  and  $\mathcal{W}^{(t-1)}$  are the current projection weight tensor and the previous projection weight tensor, respectively.

7: End

---

### B. the SPMD-LRT Based on Higher-Rank Decomposition

When  $\mathcal{W}$  has a CP decomposition of rank  $R > 1$ , i.e.  $\mathcal{W} = \sum_{r=1}^R \mathbf{v}_r^{(1)} \circ \mathbf{v}_r^{(2)} \circ \dots \circ \mathbf{v}_r^{(M)}$ , we can derive the optimization similarly by leveraging properties of CP. Following notations from Section II, let  $\mathbf{V}^{(m)} = [\mathbf{v}_1^{(m)}, \dots, \mathbf{v}_R^{(m)}] \in \mathbb{R}^{I_m \times R}$ . We use the mode- $m$  unfolding of  $\mathcal{W}$ , which can be written as  $\mathbf{W}_{(m)} = \mathbf{V}^{(m)} (\mathbf{V}^{(-m)})^T$ , where  $\mathbf{V}^{(-m)} = \mathbf{V}^{(M)} \odot \dots \odot \mathbf{V}^{(m+1)} \odot \mathbf{V}^{(m-1)} \odot \dots \odot \mathbf{V}^{(1)}$  (the Khatri-Rao product of all factor matrices except  $m$ ). Using this, one can derive analogues of Eq. (8) and (9) for CP. In particular, defining  $\tilde{\mathbf{V}}^{(m)} = \mathbf{V}^{(m)} \mathbf{A}^{1/2}$  for  $\mathbf{A} = (\mathbf{V}^{(-m)})^T \mathbf{V}^{(-m)}$  (an  $R \times R$  matrix), we obtain:

$$\begin{aligned} \langle \mathcal{W}, \mathcal{W} \rangle &= \text{tr} \left( \mathbf{w}_{(m)} \mathbf{w}_{(m)}^T \right) \\ &= \text{tr} \left( \mathbf{V}^{(m)} \left( \mathbf{V}^{(-m)} \right)^T \mathbf{V}^{(-m)} \left( \mathbf{V}^{(m)} \right)^T \right) \end{aligned} \quad (\text{B.1})$$

$$\begin{aligned} \langle \mathcal{W}, \mathcal{Z} \rangle &= \text{tr} \left( \mathbf{w}_{(m)} \mathbf{Z}_{(m)}^T \right) \\ &= \text{tr} \left( \mathbf{V}^{(m)} \left( \mathbf{V}^{(-m)} \right)^T \mathbf{Z}_{(m)}^T \right) \end{aligned} \quad (\text{B.2})$$

Where  $\mathbf{A} = (\mathbf{V}^{(-m)})^T \mathbf{V}^{(-m)}$ ,  $\tilde{\mathbf{V}}^{(m)} = \mathbf{V}^{(m)} \mathbf{A}^{1/2}$  and  $\tilde{\mathbf{Z}}^{(m)} = \mathbf{Z}_{(m)} \mathbf{V}^{(-m)} \mathbf{A}^{-1/2}$ , The Eq. (B.1) and Eq. (B.2) can be written as:

$$\begin{aligned} \langle \mathcal{W}, \mathcal{W} \rangle &= \text{tr} \left( \mathbf{w}_{(m)} \mathbf{w}_{(m)}^T \right) \\ &= \text{tr} \left( \tilde{\mathbf{V}}^{(m)} \left( \tilde{\mathbf{V}}^{(m)} \right)^T \right) \\ &= \text{vec} \left( \tilde{\mathbf{V}}^{(m)} \right)^T \text{vec} \left( \tilde{\mathbf{V}}^{(m)} \right) \\ &= \left( \mathbf{v}^{(m)} \right)^T \mathbf{v}^{(m)} \end{aligned} \quad (\text{B.3})$$

$$\begin{aligned} \langle \mathcal{W}, \mathcal{Z} \rangle &= \text{tr} \left( \tilde{\mathbf{V}}^{(m)} \left( \tilde{\mathbf{Z}}^{(m)} \right)^T \right) \\ &= \text{vec} \left( \tilde{\mathbf{V}}^{(m)} \right)^T \text{vec} \left( \tilde{\mathbf{Z}}^{(m)} \right) \\ &= \left( \mathbf{v}^{(m)} \right)^T \mathbf{Z}^{(m)} \end{aligned} \quad (\text{B.4})$$

Where  $\text{vec} \left( \tilde{\mathbf{V}}^{(m)} \right) = \mathbf{v}^{(m)}$  and  $\text{vec} \left( \tilde{\mathbf{Z}}^{(m)} \right) = \mathbf{Z}^{(m)}$ . Substituting Eq. (B.4) into Eq. (5) and (6), the margin mean  $\gamma_m$  and the margin variance  $\gamma_v$  becomes:

$$\begin{aligned} \gamma_m &= \frac{1}{N} \sum_{i=1}^N t_i \langle \mathcal{W}, \mathcal{Z}_i \rangle \\ &= \frac{1}{N} \sum_{i=1}^N t_i \left( \mathbf{v}^{(m)} \right)^T \mathbf{Z}_i^m \\ &= \frac{1}{N} \left( \mathbf{Z}^m \mathbf{t} \right)^T \mathbf{v}^{(m)} \end{aligned} \quad (\text{B.5})$$

$$\begin{aligned} \gamma_v &= \frac{1}{N} \sum_{i=1}^N (t_i \langle \mathcal{W}, \mathcal{Z}_i \rangle - \gamma_m)^2 \\ &= \frac{1}{N} \sum_{i=1}^N (t_i \langle \mathcal{W}, \mathcal{Z}_i \rangle)^2 - \left( \frac{1}{N} \sum_{i=1}^N t_i \langle \mathcal{W}, \mathcal{Z}_i \rangle \right)^2 \\ &= \left( \mathbf{v}^{(m)} \right)^T \mathbf{Z}^m \frac{N\mathbf{I} - \mathbf{t}\mathbf{t}^T}{N^2} (\mathbf{Z}^m)^T \mathbf{v}^{(m)} \end{aligned} \quad (\text{B.6})$$

Where  $\mathbf{Z}^m = [\mathbf{Z}_1^m, \dots, \mathbf{Z}_N^m]$  and  $\mathbf{t} = [t_1, \dots, t_N]$ . Substituting Eq. (B.3), Eq. (B.4), Eq. (B.5) and Eq. (B.7) into Eq. (7), the problem becomes:

$$\begin{aligned} \min_{\mathbf{v}^{(m)}, \boldsymbol{\tau}} \quad & \frac{1}{2} \left( \mathbf{v}^{(m)} \right)^T \mathbf{v}^{(m)} + \left( \mathbf{v}^{(m)} \right)^T \mathbf{Z}^m \frac{\mu_1 (N\mathbf{I} - \mathbf{t}\mathbf{t}^T)}{N^2} (\mathbf{Z}^m)^T \mathbf{v}^{(m)} \\ & - \frac{\mu_2}{N} (\mathbf{Z}^m \mathbf{t})^T \mathbf{v}^{(m)} + \frac{\lambda}{N} \mathbf{e}^T \boldsymbol{\tau} \\ \text{s.t.} \quad & \mathbf{T} (\mathbf{Z}^m)^T \mathbf{v}^{(m)} \geq \mathbf{e} - \boldsymbol{\tau}, \boldsymbol{\tau} \geq 0 \end{aligned} \quad (\text{B.7})$$

where  $\mathbf{e}$  is all-one vector. Introducing the Lagrangian multipliers  $\alpha \geq 0$  and  $\beta \geq 0$ , the Lagrangian result of Eq. (B.7) is as follows:

$$L = \frac{1}{2} \left( \mathbf{v}^{(m)} \right)^T \mathbf{S} \mathbf{v}^{(m)} - \left( \mathbf{v}^{(m)} \right)^T \mathbf{Z}^m \mathbf{T} \left( \frac{\mu_2}{N} \mathbf{e} + \boldsymbol{\alpha} \right) + \boldsymbol{\alpha}^T \mathbf{e} + \boldsymbol{\tau}^T \left( \frac{\lambda}{N} \mathbf{e} - \boldsymbol{\alpha} - \boldsymbol{\beta} \right) \quad (\text{B.8})$$

where  $\mathbf{S} = \mathbf{I} + \mathbf{Z}^m \frac{2\mu_1(N\mathbf{I} - \mathbf{t}\mathbf{t}^T)}{N^2} (\mathbf{Z}^m)^T$ . By setting the partial derivative of  $\{\mathbf{v}^{(m)}, \boldsymbol{\tau}\}$  to zero, we have:

$$\mathbf{v}^{(m)} = \mathbf{S}^{-1} \mathbf{Z}^m \mathbf{T} \left( \frac{\mu_2}{N} \mathbf{e} + \boldsymbol{\alpha} \right), 0 \leq \boldsymbol{\alpha} \leq \frac{\lambda}{N} \mathbf{e} \quad (\text{B.9})$$

By substituting Eq. (B.9) into Eq. (B.8), the dual of Eq. (B.7) can be cast as:

$$\begin{aligned} \min_{\boldsymbol{\alpha}} \quad & \frac{1}{2} \left( \frac{\mu_2}{N} \mathbf{e} + \boldsymbol{\alpha} \right)^T \mathbf{T} (\mathbf{Z}^m)^T \mathbf{S}^{-1} \mathbf{Z}^m \mathbf{T} \left( \frac{\mu_2}{N} \mathbf{e} + \boldsymbol{\alpha} \right) - \boldsymbol{\alpha}^T \mathbf{e} \\ \text{s.t.} \quad & 0 \leq \boldsymbol{\alpha} \leq \frac{\lambda}{N} \mathbf{e} \end{aligned} \quad (\text{B.10})$$

According to the Sherman-Morrison-Woodbury formula, we have

$$\mathbf{S}^{-1} \mathbf{Z}^m = \mathbf{Z}^m (\mathbf{I} + \mathbf{Q}\mathbf{G})^{-1} \quad (\text{B.11})$$

where  $\mathbf{Q} = \frac{2\mu_1(N\mathbf{I} - \mathbf{t}\mathbf{t}^T)}{N^2}$  and  $\mathbf{G} = (\mathbf{Z}^m)^T \mathbf{Z}^m$ . Then  $(\mathbf{Z}^m)^T \mathbf{S}^{-1} \mathbf{Z}^m = \mathbf{G} (\mathbf{I} + \mathbf{Q}\mathbf{G})^{-1}$ . By denoting  $\mathbf{H} = \mathbf{T}\mathbf{G}(\mathbf{I} + \mathbf{Q}\mathbf{G})^{-1} \mathbf{T}$ , the objective function of Eq. (B.10) can be written as

$$f(\boldsymbol{\alpha}) = \frac{1}{2} \boldsymbol{\alpha}^T \mathbf{H} \boldsymbol{\alpha} + \left( \frac{\mu_2}{N} \mathbf{H} \mathbf{e} - \mathbf{e} \right)^T \boldsymbol{\alpha} + \text{const} \quad (\text{B.12})$$

After eliminating the constant term, which does not influence the optimization process, the final form of the SPMD-LRT is presented as follows:

$$\begin{aligned} \min_{\boldsymbol{\alpha}} \quad & \frac{\boldsymbol{\alpha}^T \mathbf{H} \boldsymbol{\alpha}}{2} + \left( \frac{\mu_2}{N} \mathbf{H} \mathbf{e} - \mathbf{e} \right)^T \boldsymbol{\alpha} \\ \text{s.t.} \quad & 0 \leq \boldsymbol{\alpha} \leq \frac{\lambda}{N} \mathbf{e} \end{aligned} \quad (\text{B.13})$$

The coefficient  $\mathbf{w}^{(m)}$  can be derived from the result  $\boldsymbol{\alpha}^*$  of the optimization problem Eq. (B.13) as follows:

$$\mathbf{v}^{(m)} = \mathbf{Z}^m (\mathbf{I} + \mathbf{Q}\mathbf{G})^{-1} \mathbf{T} \left( \frac{\mu_2}{N} \mathbf{e} + \boldsymbol{\alpha}^* \right) = \mathbf{Z}^m \mathbf{u} \quad (\text{B.14})$$

Where  $\mathbf{u} = (\mathbf{I} + \mathbf{Q}\mathbf{G})^{-1} \mathbf{T} \left( \frac{\mu_2}{N} \mathbf{e} + \boldsymbol{\alpha}^* \right)$ . It should be mentioned here that the whole procedure is also repeated iteratively for every mode. The pseudo-code for the SPMD-LRT based on the Higher-Rank decomposition (HSPMD-LRT) is provided in Algorithm 3.

---

**Algorithm 2** HSPMD-LRT Algorithm
 

---

Input: Training dataset  $\left\{ \mathcal{Z}_i \in \mathbb{R}^{I_1 \times I_2 \times \dots \times I_M}, \mathbf{t}_i \in \{-1, 1\}_{i=1}^N \right\}$ , Parameters:  $\mu_1, \mu_2, \lambda$

Output:  $\mathcal{W}$

Steps:

- 1: Set  $\mathbf{V}^{(m)}$  equal to random unit matrices in  $\mathbb{R}^{I_m \times R}$ .
- 2: Do Steps 3-5 until convergence.
- 3: For  $m = 1$  to  $M$
- 4: Update  $\mathbf{V}^{(m)}$  by the following question

$$\begin{aligned} \min_{\boldsymbol{\alpha}} \quad & \frac{\boldsymbol{\alpha}^T \mathbf{H} \boldsymbol{\alpha}}{2} + \left( \frac{\mu_2}{N} \mathbf{H} \mathbf{e} - \mathbf{e} \right)^T \boldsymbol{\alpha} \\ \text{s.t.} \quad & 0 \leq \boldsymbol{\alpha} \leq \frac{\lambda}{N} \mathbf{e} \end{aligned}$$

Where  $\mathbf{v}^{(m)} = \mathbf{Z}^m (\mathbf{I} + \mathbf{Q}\mathbf{G})^{-1} \mathbf{T} \left( \frac{\mu_2}{N} \mathbf{e} + \boldsymbol{\alpha}^* \right)$ ,  $\tilde{\mathbf{V}} = \text{reshape}(\mathbf{v}^{(m)})$  and  $\mathbf{V}^{(m)} = \tilde{\mathbf{V}}^{(m)} \mathbf{A}^{-\frac{1}{2}}$

5: End For

6: Convergence checking:

$$\text{if } \left\| \mathcal{W}^{(t)} - \mathcal{W}^{(t-1)} \right\| / \left\| \mathcal{W}^{(t-1)} \right\| \leq \varepsilon$$

Where  $\mathcal{W} = \sum_{r=1}^R \mathbf{v}_r^{(1)} \circ \mathbf{v}_r^{(2)} \circ \dots \circ \mathbf{v}_r^{(M)} = \llbracket \mathbf{V}^{(1)}, \mathbf{V}^{(2)}, \dots, \mathbf{V}^{(M)} \rrbracket$ , the calculate  $\mathbf{V}^{(m)}, m = 1, 2, \dots, M$  have converged. Here  $\mathcal{W}^{(t)}$  and  $\mathcal{W}^{(t-1)}$  are the current projection weight tensor and the previous projection weight tensor, respectively.

7: End

---

### C. Proofs of Theoretical Results

This appendix provides the detailed proofs of the lemmas and theorems stated in Section IV.

- Proof of Lemma 1

Proof. Let  $\mathcal{W} = \llbracket \mathcal{F}, V^{(1)}, \dots, V^{(M)} \rrbracket$  be a Tucker decomposition. For any mode- $m$  unfolding,

$$\mathcal{W}_{(m)} = V^{(m)} F_{(m)} (V^{(-m)})^\top, \quad (\text{C.1})$$

where  $V^{(-m)}$  denotes the Kronecker product of all  $V^{(j)}$  with  $j \neq m$ . Then,

$$\|\mathcal{W}\|_F = \|\mathcal{W}_{(m)}\|_F \quad (\text{C.2})$$

$$\leq \|V^{(m)}\|_2 \|F_{(m)}\|_F \|V^{(-m)}\|_2, \quad (\text{C.3})$$

by submultiplicativity of the Frobenius and operator norms. Since  $\|F_{(m)}\|_F = \|\mathcal{F}\|_F$ , the result follows:

$$\|\mathcal{W}\|_F \leq \|\mathcal{F}\|_F \prod_{m=1}^M \|V^{(m)}\|_2.$$

□

- Proof of Lemma 2

Proof. Consider the Rademacher complexity

$$\mathfrak{R}_N(\mathcal{H}_B) = \frac{1}{N} \mathbb{E}_\sigma \left[ \sup_{\|\mathcal{W}\|_F \leq B} \sum_{i=1}^N \sigma_i \langle \mathcal{W}, \mathcal{Z}_i \rangle \right] \quad (\text{C.4})$$

$$= \frac{1}{N} \mathbb{E}_\sigma \left[ \sup_{\|\mathcal{W}\|_F \leq B} \langle \mathcal{W}, \sum_{i=1}^N \sigma_i \mathcal{Z}_i \rangle \right]. \quad (\text{C.5})$$

By Cauchy-Schwarz inequality,

$$\sup_{\|\mathcal{W}\|_F \leq B} \langle \mathcal{W}, \mathcal{A} \rangle = B \|\mathcal{A}\|_F. \quad (\text{C.6})$$

Therefore,

$$\mathfrak{R}_N(\mathcal{H}_B) = \frac{B}{N} \mathbb{E}_\sigma \left\| \sum_{i=1}^N \sigma_i \mathcal{Z}_i \right\|_F. \quad (\text{C.7})$$

Since  $\|\mathcal{Z}_i\|_F \leq R$ , we bound

$$\mathbb{E}_\sigma \left\| \sum_{i=1}^N \sigma_i \mathcal{Z}_i \right\|_F^2 = \mathbb{E}_\sigma \left[ \sum_{i=1}^N \sum_{j=1}^N \sigma_i \sigma_j \langle \mathcal{Z}_i, \mathcal{Z}_j \rangle \right] \quad (\text{C.8})$$

$$= \sum_{i=1}^N \|\mathcal{Z}_i\|_F^2 \leq NR^2. \quad (\text{C.9})$$

Taking square roots,

$$\mathbb{E}_\sigma \left\| \sum_{i=1}^N \sigma_i \mathcal{Z}_i \right\|_F \leq R\sqrt{N}.$$

Thus,

$$\mathfrak{R}_N(\mathcal{H}_B) \leq \frac{BR}{\sqrt{N}}.$$

□

- Proof of Theorem 1: Cantelli Bound

Proof. Let the random variable  $M = t\langle \mathcal{W}, \mathcal{Z} \rangle$  denote the margin. Define  $\mu = \gamma_m = \mathbb{E}[M]$  and  $\sigma^2 = \gamma_v = \text{Var}(M)$ . For any  $\rho < \mu$ , consider

$$\Pr(M \leq \rho) = \Pr(M - \mu \leq \rho - \mu).$$

Since  $\rho - \mu < 0$ , Cantelli's inequality (one-sided Chebyshev bound) gives

$$\Pr(M - \mu \leq \rho - \mu) \leq \frac{\sigma^2}{\sigma^2 + (\mu - \rho)^2}.$$

Therefore,

$$\Pr(M \leq \rho) \leq \frac{\gamma_v}{\gamma_v + (\gamma_m - \rho)^2}.$$

□

- Proof of Theorem 2

Proof. (1) Monotonic descent. At each iteration, one block (e.g.,  $V^{(m)}$ ,  $\mathcal{F}$ , or  $\tau$ ) is updated by solving a convex quadratic program (QP) with all other variables fixed. Each subproblem is solved to its global minimum, so the objective  $J$  cannot increase. Therefore, the sequence  $\{J_k\}$  is monotonically non-increasing.

(2) Boundedness. Since  $J$  is lower-bounded by 0, the sequence  $\{J_k\}$  is bounded from below. Furthermore, the regularization term  $\frac{1}{2}\|\mathcal{W}\|_F^2$  prevents  $\|\mathcal{W}\|_F$  from diverging. Consequently, the iterates  $\{V_k^{(m)}, \mathcal{F}_k, \tau_k\}$  remain bounded.

(3) Convergence to a stationary point. The objective  $J$  is a semi-algebraic function (constructed from polynomial and norm terms), which satisfies the Kurdyka-Łojasiewicz (KL) property. By standard results on block coordinate descent (BCD) methods for KL functions, any bounded sequence generated by exact block updates converges to a critical point (stationary point) of  $J$ . □
